# Supplementary material for: Whitening-based Contrastive Learning of Sentence Embeddings
Source: arXiv:2305.17746 source file (2023-06-08)
Supplement: Supplementary file 1 [file appendix.tex]

\appendix

\section{Example Appendix}
\label{sec:appendix}

This is an appendix.
